# Supplementary material for: Direct observation of charge mediated lattice distortions in complex oxide solid solutions
Source: arXiv:1409.4432 source file (2014-09-15)
Supplement: Supplementary file 1 [file supplement.pdf]

# Supplemental Material for: Direct observation of charge mediated lattice distortions in complex oxide solid solutions

Xiahan Sang, Everett D. Grimley, Changning Niu, Douglas L. Irving, James M. LeBeau

*Department of Materials Science & Engineering, North Carolina State University**

(Dated: September 15, 2014)

**RevSTEM method and complete RevSTEM image**

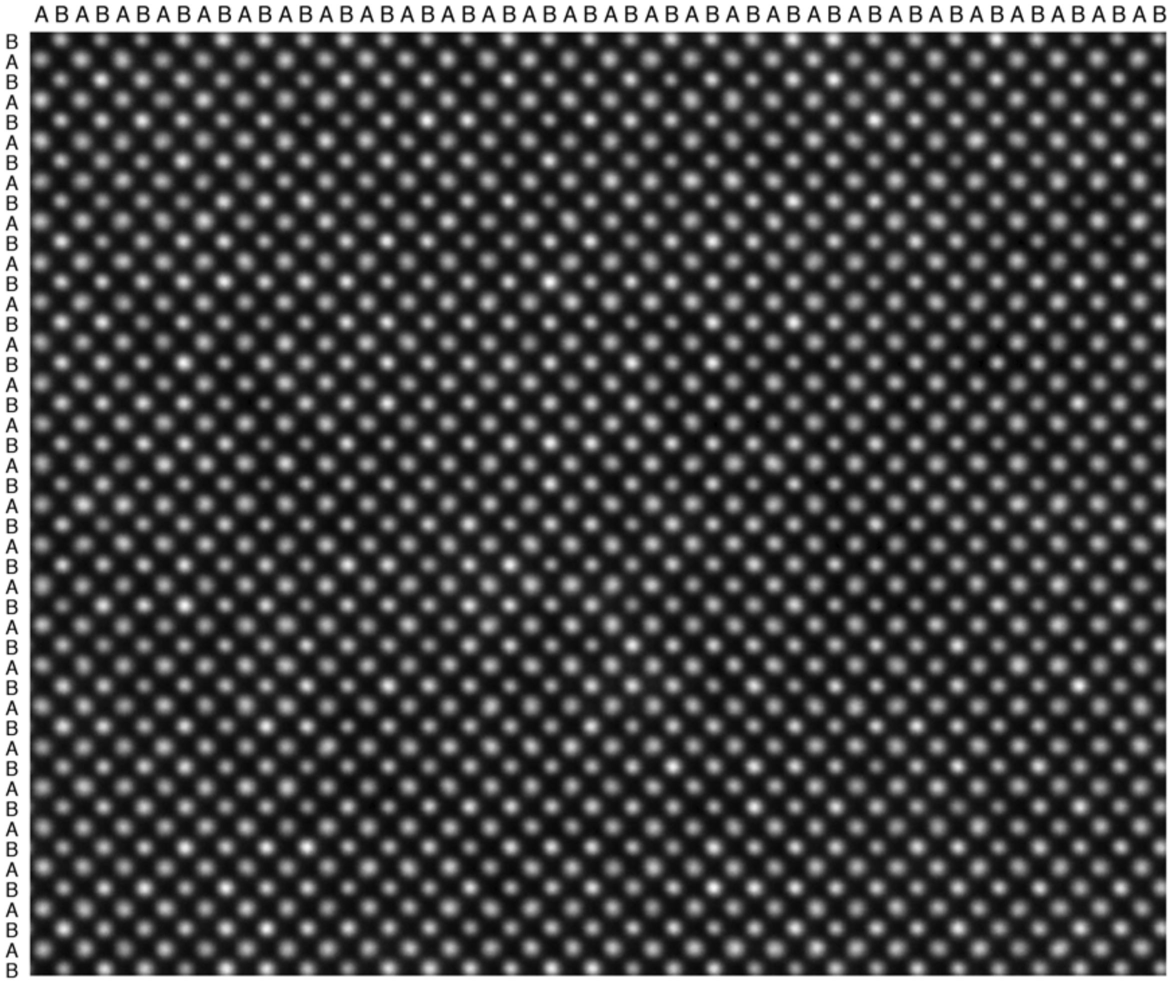


FIG. 1. The complete LSAT RevSTEM image used for analysis, which was representative for the sample.

$(La_{0.18}Sr_{0.82})(Al_{0.59}Ta_{0.41})O_3$ and Si (MTI Corporation Richmond, CA) single crystals were prepared for electron microscopy by mechanical wedge polishing with an Allied Multi-prep [1]. Imaging was performed using a probe-corrected FEI Titan G2 60-300kV S/TEM equipped with an X-FEG source operated at 200 kV. The convergence and collection inner semi-angles were 15 mrad and 77 mrad respectively for HAADF STEM images and the probe current was approximately 60–100 pA as measured by the screen current monitor. A custom program was used to acquire the RevSTEM image series by interfacing with the microscope through TEM Imaging and Analysis (TIA) [2]. For both LSAT and Si HAADF

RevSTEM datasets, 40 $1024 \times 1024$ images were acquired with a dwell time of 2 $\mu$s/pixel. The rotation angle between successive image frames was 90°. The LSAT RevSTEM dataset was calibrated using the known lattice constant of 386.8 pm . Each atom column position was determined by fitting the corresponding image intensities to a two-dimensional Gaussian function. Further details on image accuracy and fit precision are provided in the subsection **Atom column distance measurements: accuracy and precision** in this Supplemental Material.

### DFT Calculations and DFT Structures

First principles simulations were performed with the well established plane wave Vienna Ab initio Software Package (VASP) version 5.3.3 [3–6]. In all calculations, the electrons were handled within the projector augmented wave pseudopotentials that were provided with the VASP distribution [7, 8]. For La, Sr, Al, Ta and O atoms, 11, 10, 3, 5, and 6 electrons were treated as valence, respectively. The minimized geometries were determined by a conjugate gradient algorithm that ended when all forces were below 0.01 eV/Å with the electronic convergence per step set below $10^{-8}$ eV/atom. Two different k-point meshes were used during the simulation. Initial relaxations used the $\gamma$ point. After these converged completed, a higher k-point density was selected to be above 500 k-points per reciprocal atom. In all simulations the kinetic energy cutoff was set to 500 eV due to the presence of oxygen. The exchange correlation functional was the gradient corrected functional of Perdew, Burke, and Ernzerhof (PBE) [9, 10]. Due to the presence of transition metals, the spherically averaged +U approximation of Dudarev [11] was applied to the PBE functional with values of U, in this case $U_{\text{eff}}$ equal to U-J, taken from the literature [12].

Multiple special quasi random structures for LSAT were evaluated. Two different structures were used to simulate the LSAT structure. Both were special quasi-random structures [13] generated using the Monte Carlo algorithm [14] within the Alloy Theoretic Automated Toolkit (ATAT) [15–17]. One structure was the best SQS for any super cell symmetry based on what minimized both pair and multi-site correlation functions. The second structure also used the SQS framework but limited the search for the most random site population in a *cubic* crystal structure. Both structures had a total of 135 atoms per super cell with 5 La, 22 Sr, 16 Al, 11 Ta, and 81 O. This results in a total composition of $(La_{0.185}Sr_{0.815})(Al_{0.593}Ta_{0.407})O_3$

that compares to the experimental composition. The cubic SQS structure was found to have the lowest total energy by greater than 50 meV/formula unit. The $3 \times 3 \times 3$ cubic structure as shown in Figure 1A of the manuscript was selected as more representative due to its lower energy but more detailed simulations are required to determine the structure that fully minimizes the free energy of the structure. This effort is outside of the scope of the present work.

In an effort to quantify the degree of charge on each atom, we selected the use of the Bader charge formalism [18, 19]. Within this formalism the real space electron densities are divided into sub-volumes based on special zero flux points in the self-consistently converged electron density. All Bader charges were tested at multiple FFT mesh densities and k-point densities for convergence. All charges reported here were converged to the order of 0.01 $e^-$ per ion. Table I shows the charge in the unrelaxed and relaxed structures along with the standard deviation and number of atoms in each sub-group. There is a small change in charge as the structure relaxes but none of the discussed trends change as a result of these changes.

TABLE I. Bader charges determined before (initial) and after (final) DFT structure relaxation.

| Atom | $q_{initial}$ | $q_{final}$ | Number of Atoms |
|---|---|---|---|
| La | 2.04±0.02 | 2.14±0.02 | 5 |
| Sr | 1.56±0.01 | 1.58±0.00 | 22 |
| Al | 2.43±0.01 | 2.47±0.01 | 16 |
| Ta | 2.54±0.01 | 2.55±0.01 | 11 |
| O (Total) | -1.37±0.11 | -1.40±0.13 | 81 |
| O (Al-O-Al) | -1.51±0.01 | -1.56±0.02 | 28 |
| O (Al-O-Ta) | -1.33±0.02 | -1.34±0.02 | 40 |
| O (Ta-O-Ta) | -1.23±0.01 | -1.21±0.02 | 13 |

## STEM Image Simulations

The relaxed crystal structure projected along three different $\langle 100 \rangle$ orientations (Figure 2A) reveals that the A sub-lattice exhibits significant deviation from the averaged positions as compared to the B-sub lattice. Simulated STEM images of the DFT-relaxed $3 \times 3 \times 3$ supercell were generated along the three $\langle 100 \rangle$ orientations using the frozen phonon multislice algorithm with parameters matching the experimental conditions [20] (Fig. 2). Additionally, we also simulated a $3 \times 3 \times 9$ supercell combining the three $\langle 100 \rangle$ zones axes aligned to a common direction. The projected potentials were sampled at 3.46 pm/pixel and were used to simulate a $3 \times 3$ unit-cells STEM images with $30 \times 30$ probe positions. The simulated sample thickness was 14.2 nm, closely matching that of experiment ($14 \pm 1$ nm) as determined using position averaged convergent beam electron diffraction [21]. The simulated data was enlarged using Fourier interpolation and blurred with a Gaussian function of 0.10 nm to approximately account for the finite size of the electron probe [22].

Simulated HAADF STEM images are shown in Figure 2B where the color of the rounded squares indicate the average NLN around the A and B sub-lattices. The resulting almost uniform distance between B-B NLN and varying distance between A-A NLN in the simulation supports the results of the experimental STEM images. The contraction of unit cell around darker B sub-lattice (Al rich) and expansion of unit cell around brighter B sub-lattice (Ta rich) agree well with experiment for each simulation.

## The correlation coefficient

Following the discussion in Ref. [23, 24], the correlated distortion of atom column pairs can be described by:

$$\phi = \frac{\sigma_0^2 - \sigma^2}{2\sigma_0^2} \tag{1}$$

where $\sigma$ is the measured standard deviation for each atom column pair on a particular sub-lattice and $\phi$ is the correlation coefficient for $n^{th}$ like-neighbor distances as applied to describe the effects of correlated motion in PDF analysis [23, 25]. The parameter $\sigma_0$ represents the contribution from uncorrelated distortion and can be extracted at large distances where the uncorrelated distortion dominates, i.e. when $\phi \sim 0$. Here we use the average from $2 < r < 5$

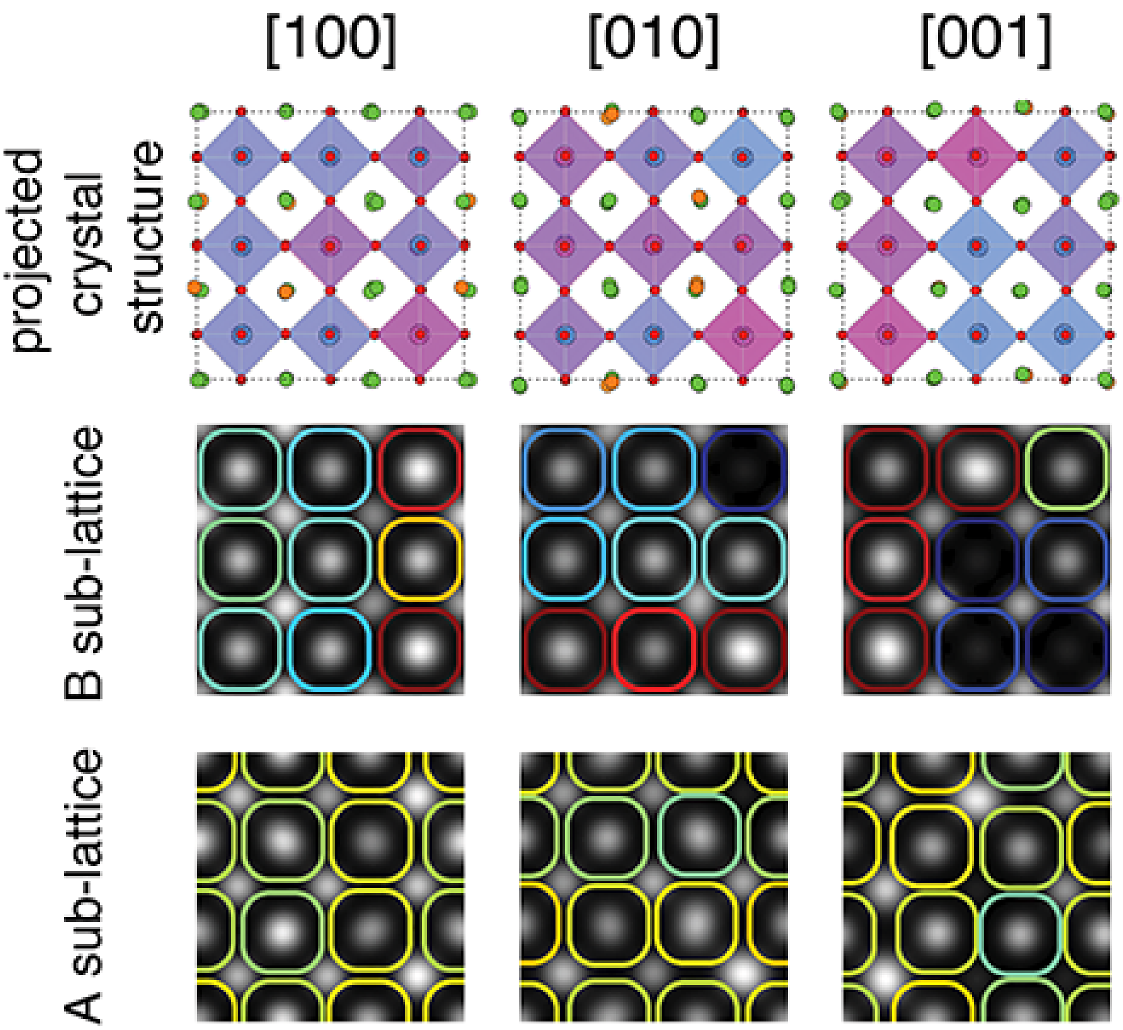


FIG. 2. The projected DFT-relaxed $3 \times 3 \times 3$ LSAT supercell along [100], [010] and [001] zone axes. Simulated HAADF STEM image are shown with rounded squares with color indicating the length of the average NLN around each B sub-lattice atom simulated LSAT HAADF STEM image . (C) Rounded squares with color indicating the length of the average NLN around each A sub-lattice atom. The same color scheme as in Figure 1 D and E of the manuscript.

nm where $\sigma_0^A$ and $\sigma_0^B$ are 6.5 pm and 3.9 pm respectively. Note that the correlated distortion in STEM images arises only from static displacements, as dynamic motion due to phonons is averaged out.

As demonstrated in the manuscript, A sub-lattice distortion is triggered by charge fluctuation on the B sub-lattice. For Al deficient B sub-lattice atom columns, the movement of atoms can be schematically represented in Figure 3 (also shown in Figure 3E of the

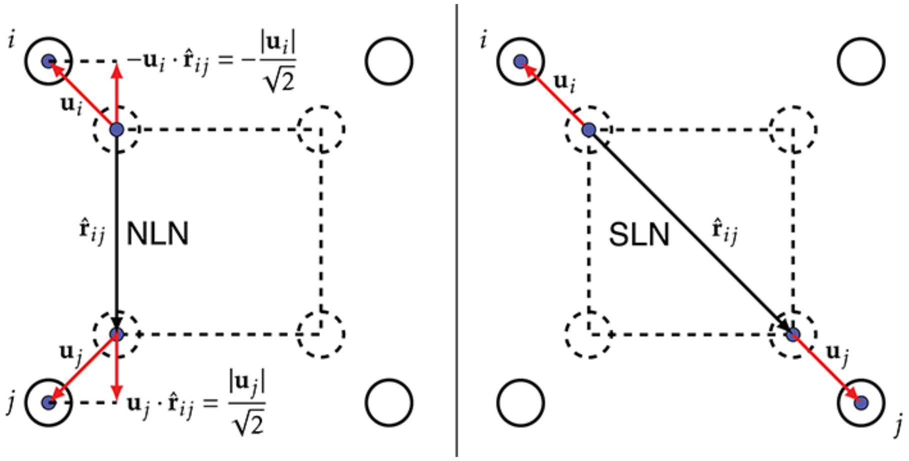


FIG. 3. Schematic representation of the influence of anti-correlated distortion on the first and second like-neighbor distance measurements.

manuscript). Note that $\mathbf{u}_i$ and $\mathbf{u}_j$ are the displacements of atoms $i$ and $j$ (indicated by red vectors in Fig. 3) from their ideal positions and $\mathbf{r}_{ij}$ is the unit vector defining the angle from atom $i$ to atom $j$. For the atom pair $i$ and $j$, the correlation coefficient for the NLN is given by $(\mathbf{u}_i \cdot \hat{\mathbf{r}}_{ij})(\mathbf{u}_j \cdot \hat{\mathbf{r}}_{ij}) =$ -$\frac{|\mathbf{u}_i|}{\sqrt{2}} \frac{|\mathbf{u}_j|}{\sqrt{2}} = -|\mathbf{u}_i||\mathbf{u}_j|/2$. In contrast for the SLN, $\mathbf{r}_{ij}$ is parallel to $\mathbf{u}_i$ and $\mathbf{u}_j$, yielding a correlation contribution $-|\mathbf{u}_i||\mathbf{u}_j|$. Thus, the NLN and SLN correlation coefficients are both negative, with a larger magnitude for the SLN.

### Atom column distance measurements: accuracy and precision

While the RevSTEM method eliminates distortion caused by sample drift, other types of distortion in the scan system can remain. In particular, slight mis-calibration of the scan system introduces additional global distortion that results in skewing, expansion, and/or contraction of the unit cells of the image. At lower magnification, the scan coordinate distortion can be corrected using a standard square grating [2], however, this approach was found to be insufficient to consistently remove minute residual distortion for atomic scale imaging. To determine the affine coefficients ($x_1$, $x_2$ and $x_3$), we apply a least squares regression that minimizes $\chi^2 = \sum_i \sigma_i^2$ using a calibration image of $\langle 100 \rangle$ Si. After applying the global distortion correction transformation, $\sigma$ is rendered stable for distances that span the image as shown in Manuscript Figure 3d where 2 pm precision for Si holds up to about 5 nm.

Quantitative distance analysis also requires accurate and precise determination of the location of atom columns in the RevSTEM images. Importantly, the RevSTEM images contain negligible distortion and possess a high signal to noise ratio; these characteristics enable direct fitting of two-dimensional Gaussian functions to the experimental atom columns. A two-dimensional Gaussian distribution with adjustable variables including position, peak intensity, background intensity, widths at two principle axes and rotation angle was used to fit the intensity of every atom column. The initial values for atom column positions were located by a normalized cross-correlation approach similar to that in Ref. [26].

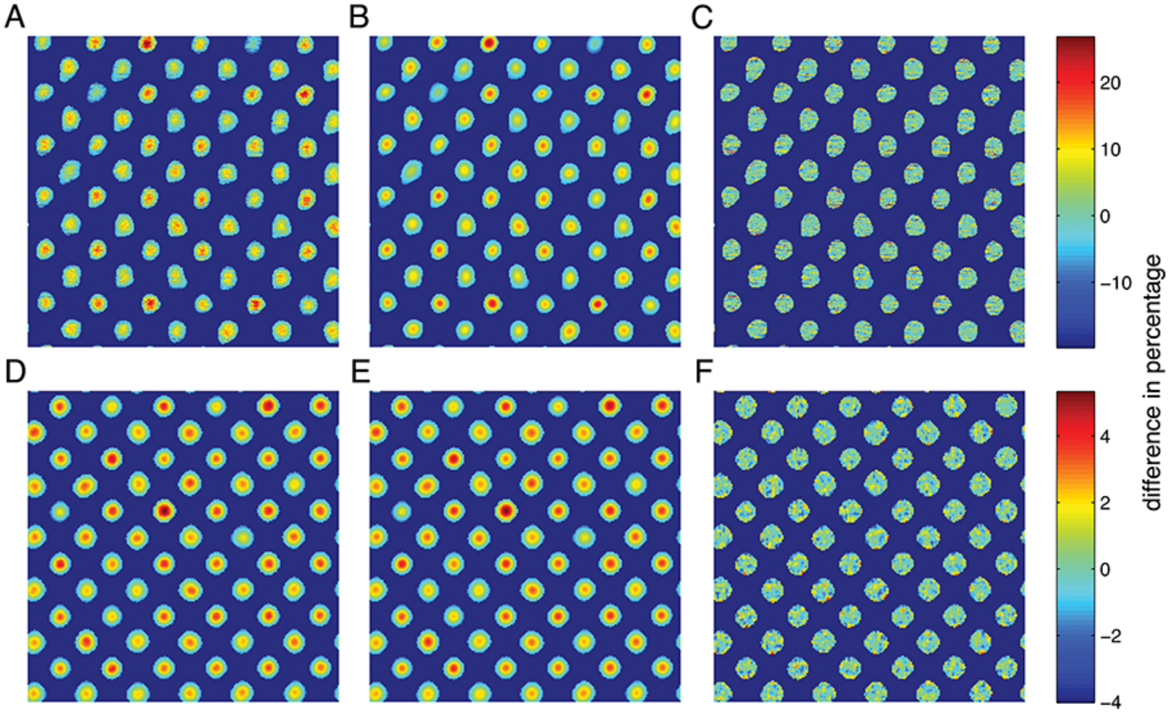


FIG. 4. (A) Masked atom column locations for a sub-region of a conventional STEM image. (B) Intensity distribution from two-dimensional Gaussian fitting. (C) The difference between (A) and (B). (D) Masked atom column locations for a sub-region of a RevSTEM image. (E) Intensity distribution from two-dimensional Gaussian fitting. (F) The difference between (D) and (E).

For comparison, Figure 4 A-C shows the resulting fit first using a conventional STEM image acquired with a 12 $\mu$s dwell time. While the fit appears satisfactory, significant horizontal image tearing is evident in the experimental image, Figure 4A, and in the difference map, Figure 4C. The tearing effect combined with the low signal-to-noise ratio leads to resid-

ual error between experiment and fit as high as 20%. In contrast, the difference between experimental RevSTEM image, Figure 4D, and the Gaussian fit, Figure 4E, generally shows deviation less than 5% (Fig. 4F).

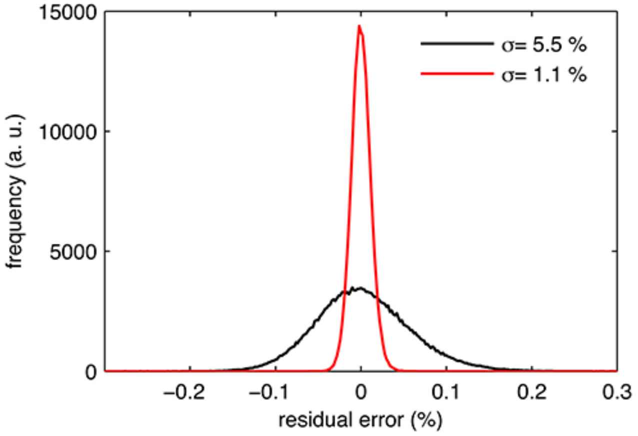


FIG. 5. Histogram of the percentage error between fits and the conventional STEM (black line) and RevSTEM (red line) images.

For a direct comparison of the residual difference, histograms for the percent error from Figures 4 C and F are shown in Figure 5. Note that standard deviation of the error is 5.5% for the conventional STEM image (black line) while this is improved by a factor of five for the RevSTEM image, $\sigma = 1.1\%$. The comparatively minor error in the RevSTEM dataset indicates a robust and reliable peak fitting result.

To further illustrate the precision, we introduced a deliberate offset between the fit and experimental data. The artificial systematic error introduces systematic asymmetry in the corresponding different maps, which is shown in Figure 6. The fit result was shifted by either 1, 2, 3, 5 or 10 pm along both horizontal and vertical directions. For the conventional STEM image, the asymmetry in the difference map is not readily observable until a shift of about 3-5 pm. In contrast, even a 1 pm shift in the RevSTEM fit data, produces a perceivable asymmetry in the deviation map that becomes more pronounced as the mismatch increases. These comparisons demonstrate that the RevSTEM method can consistently achieve atomic column location precision within the picometer regime.

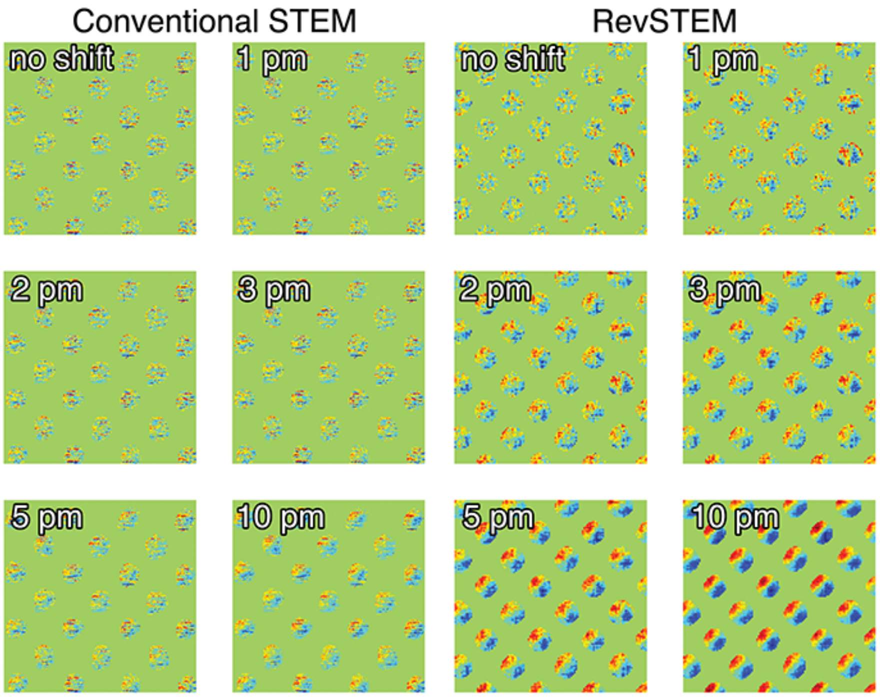


FIG. 6. The difference map between experiment and fit after a relative shift of 1 pm, 2 pm, 3 pm, 5 pm and 10 pm for both conventional and RevSTEM images.

* jmlebeau@ncsu.edu

[1] P. Voyles, J. Grazul, and D. Muller, Ultramicroscopy **96**, 251 (2003), proceedings of the International Workshop on Strategies and Advances in Atomic Level Spectroscopy and Analysis.

[2] X. Sang and J. M. Lebeau, Ultramicroscopy **138**, 28 (2014).

[3] G. Kresse and J. Hafner, Phys. Rev. B **47**, 558 (1993).

[4] G. Kresse and J. Hafner, Phys. Rev. B **49**, 14251 (1994).

[5] G. Kresse and J. Furthmüller, Computational Materials Science **6**, 15 (1996).

[6] G. Kresse and J. Furthmüller, Phys. Rev. B **54**, 11169 (1996).

[7] G. Kresse and D. Joubert, Phys. Rev. B **59**, 1758 (1999).

[8] P. E. Blöchl, Phys. Rev. B **50**, 17953 (1994).

[9] J. P. Perdew, K. Burke, and M. Ernzerhof, Phys. Rev. Lett. **77**, 3865 (1996).

[10] J. P. Perdew, K. Burke, and M. Ernzerhof, Phys. Rev. Lett. **78**, 1396 (1997).

[11] S. L. Dudarev, G. A. Botton, S. Y. Savrasov, C. J. Humphreys, and A. P. Sutton, Physical Review B **57**, 1505 (1998).

[12] W. Setyawan, R. M. Gaume, S. Lam, R. S. Feigelson, and S. Curtarolo, ACS Combinatorial Science **13**, 382 (2011).

[13] A. Zunger, S. Wei, L. Ferreira, and J. Bernard, Physical review letters **65**, 353 (1990).

[14] A. van de Walle, P. Tiwary, M. de Jong, D. Olmsted, M. Asta, A. Dick, D. Shin, Y. Wang, L.-Q. Chen, and Z.-K. Liu, Calphad **42**, 13 (2013).

[15] A. van de Walle, Calphad **33**, 266 (2009).

[16] A. van de Walle and G. Ceder, Journal of Phase Equilibria **23**, 348 (2002).

[17] A. V. D. Walle, M. Asta, and G. Ceder, Calphad **26**, 539 (2002).

[18] R. Bader, *Atoms in Molecules: A Quantum Theory*, International series of monographs on chemistry (Clarendon Press, 1990).

[19] G. Henkelman, A. Arnaldsson, and H. Jónsson, Computational Materials Science **36**, 354 (2006).

[20] E. J. Kirkland, *Advanced Computing in Electron Microscopy* (Springer US, 2010) pp. 1–4.

[21] J. M. LeBeau, S. D. Findlay, L. J. Allen, and S. Stemmer, Ultramicroscopy **110**, 118 (2010).

[22] J. LeBeau, S. Findlay, L. Allen, and S. Stemmer, Physical Review Letters **100**, 206101 (2008).

[23] I.-K. Jeong, T. Proffen, F. Mohiuddin-Jacobs, and S. J. L. Billinge, The Journal of Physical Chemistry A **103**, 921 (1999).

[24] I.-K. Jeong, R. H. Heffner, M. J. Graf, and S. J. L. Billinge, Phys. Rev. B **67**, 104301 (2003).

[25] C. H. Booth, F. Bridges, E. D. Bauer, G. G. Li, J. B. Boyce, T. Claeson, C. W. Chu, and Q. Xiong, Phys. Rev. B **52**, R15745 (1995).

[26] J.-M. Zuo, A. B. Shah, H. Kim, Y. Meng, W. Gao, and J.-L. RouviÃ©re, Ultramicroscopy **136**, 50 (2014).
